# Supplementary material for: What Can We Learn from Collective Human Opinions on Natural Language Inference Data?
Source: arXiv:2010.03532 source file (2020-10-08)
Supplement: Supplementary file 1 [file appendix_head.tex]

\documentclass[11pt,a4paper]{article}
\usepackage[hyperref]{emnlp2020}
\usepackage{times}
\usepackage{latexsym}
\usepackage{framed}
\usepackage{enumitem}
\usepackage{subcaption}
\usepackage{graphicx}
\usepackage{booktabs}
\usepackage{multirow}
\usepackage{multicol}
\usepackage{enumitem}

\usepackage{xspace}
\usepackage{amsmath}
\usepackage{amssymb}
\usepackage{subcaption}

% This is not strictly necessary, and may be commented out,
% but it will improve the layout of the manuscript,
% and will typically save some space.
\usepackage{microtype}

%\aclfinalcopy % Uncomment this line for the final submission
%\def\aclpaperid{***} %  Enter the acl Paper ID here

%need commands

\title{Appendix: What Can We Learn from Collective Human Opinions on Natural Language Inference Data?}

\date{}

\begin{document}
\maketitle

\renewcommand\thesection{\Alph{section}}
\input{supplementary/appendix_context}

\newpage

% \bibliography{emnlp2020}
% \bibliographystyle{acl_natbib}

\end{document}
